# Supplementary material for: Stripe order and magnetic anisotropy in the $S=1$ antiferromagnet BaMoP$_2$O$_8$
Source: arXiv:1806.09314 source file (2018-09-06)
Supplement: Supplementary file 1 [file Supplemental_Material.pdf]

# *Supplemental Material*
# Stripe order and magnetic anisotropy in the $S = 1$ antiferromagnet $BaMoP_2O_8$

Jan Hembacher,[1] Danis I. Badrtdinov,[1,2] Lei Ding,[1] Zuzanna Sobczak,[1,3] Clemens Ritter,[4] Vladimir V. Mazurenko,[2] and Alexander A. Tsirlin[1,2,*]

[1] *Experimental Physics VI, Center for Electronic Correlations and Magnetism, Institute of Physics, University of Augsburg, 86135 Augsburg, Germany*
[2] *Theoretical Physics and Applied Mathematics Department, Ural Federal University, 620002 Yekaterinburg, Russia*
[3] *Faculty of Applied Physics and Mathematics, Gdansk University of Technology, ul. Narutowicza 11/12, 80-233 Gdansk*
[4] *Institut Laue-Langevin, BP 156, F-38042 Grenoble, France*

Here, we provide details of the sample preparation and characterization.

Polycrystalline samples of $BaMoP_2O_8$ were synthesized using two different routes. The first route includes the reaction of $BaCO_3$ and $NH_4H_2PO_4$ in air at 600 °C for 24 hours to produce a precursor that is further mixed with the stoichiometric amount of $MoO_2$ and annealed in an evacuated and sealed quartz tube at 900 °C for 24 hours. This yields the $BaMoP_2O_8$ phase with about 10 wt.% of the $MoO_2$ impurity, which persisted even after additional annealings at an increased temperature of 930 − 950 °C. Magnetic susceptibility of such samples showed a large paramagnetic impurity contribution ("Curie tail"), and the broad maximum expected in frustrated antiferromagnets was never very pronounced (Fig. S1, sample I). This Curie tail is likely due to defects in $BaMoP_2O_8$ and unrelated to the $MoO_2$ impurity, which has a low and weakly temperature-dependent susceptibility within the temperature range of our study [1].

The second synthesis route begins with the reaction of $BaCO_3$, $NH_4H_2PO_4$, and $MoO_3$ in air at 600° for 24 hours, where the amount of $MoO_3$ is two thirds of the stoichiometric amount of molybdenum in $BaMoP_2O_8$. The resulting precursor is mixed with metallic molybdenum and annealed in an evacuated and sealed quartz tube at 900 °C for 24 hours [2]. Molybdenum powder should be sufficiently active for completing this reaction. For example, the powder with the grain size of 100 $\mu$m (325 mesh) produced a multi-phase mixture, and the reaction was clearly incomplete. On the other hand, the $2-4$ $\mu$m powder proved to produce the $BaMoP_2O_8$ phase with only minor amounts of the Mo and $MoO_2$ impurities. Similar to the first synthesis route, neither Mo nor $MoO_2$ should have affected the magnetic susceptibility, but a pronounced Curie-like impurity contribution was again observed, whereas the broad maximum remained largely smeared out (Fig. S1, sample II). This problem could be remedied by adding the two-fold to three-fold excess of metallic molybdenum. Excess Mo was then washed out by 23 % $HNO_3$ after the synthesis. The resulting samples showed a pronounced susceptibility maximum (Fig. S1, sample III) and were used in subsequent thermodynamic measurements.

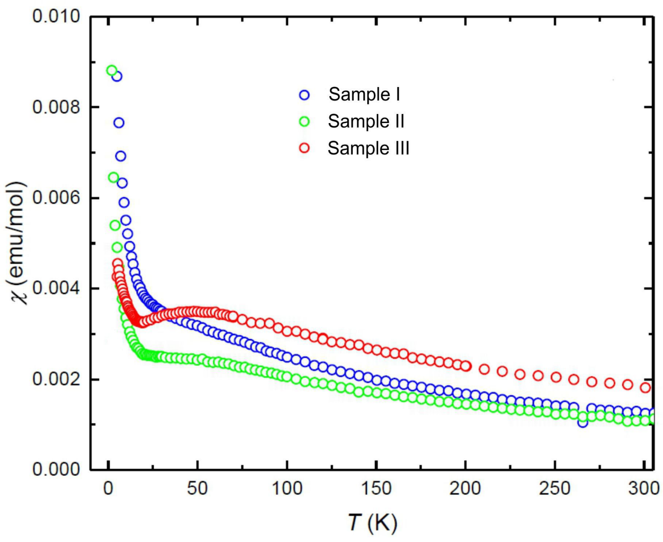


FIG. S1. Magnetic susceptibility of three samples prepared under different synthesis conditions, as explained in the text and in the caption of Table S1. Samples I and II were measured with an applied magnetic field of 0.05 T. Sample III was measured with an applied magnetic field of 0.1 T.

Rietveld refinement (Table S1) did not reveal any significant structural differences between the samples obtained via different synthesis routes or with and without excess Mo. The lattice parameters and reflection widths were very similar in all samples. Presently, we are unable to conclude which sample feature is responsible for the Curie-like impurity contribution. It seems plausible that extra metallic molybdenum may be needed to ensure the lower oxygen pressure during the reaction and the complete reduction toward $Mo^{4+}$, but detailed study of this issue goes beyond the scope of our present work. We also note that $BaMoP_2O_8$ melts congruently around 1000 °C, but crystal growth from the melt was so far unsuccessful.

* altsirlin@gmail.com

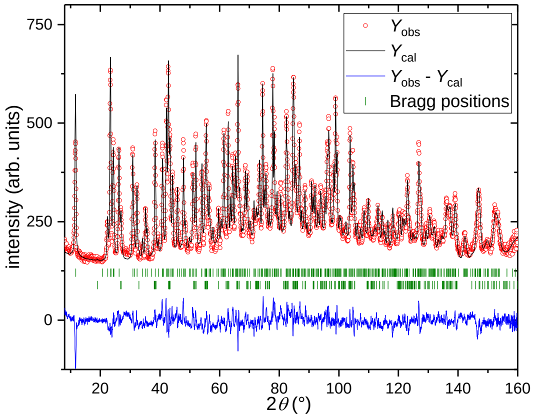


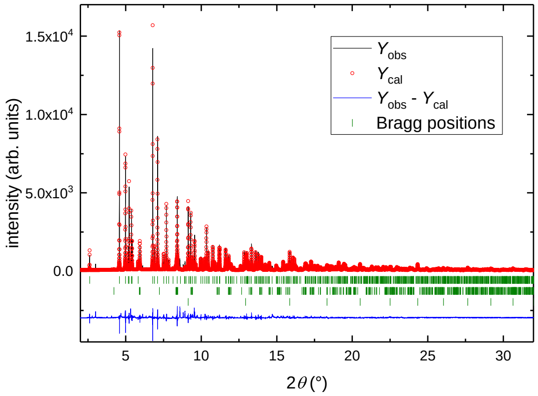


FIG. S2. Rietveld refinement for $BaMoP_2O_8$: room-temperature neutron data (left) and 20 K synchrotron data (right). The tick marks denote the Bragg-peak positions for $BaMoP_2O_8$ (first row) and $MoO_2$ (second row). In the right panel, the third row of tick marks stands for the peak positions of the metallic molybdenum that was present in a very tiny amount (well below 1 wt.%) even after the $HNO_3$ treatment.

[1] J. Ghose, N. N. Greenwood, G. C.Hallam, and D. A. Read, "Neutron diffraction study of molybdenum dioxide," J. Solid State Chem. **19**, 365–368 (1976).

[2] Similar results were obtained when quartz tubes were filled with 100 mbar of Ar.

TABLE S1. Refined lattice parameters, atomic positions and profile parameters (Lorentzian, in $10^{-2}$ deg) at room temperature for three samples prepared under different synthesis conditions: sample I was obtained from $MoO_2$, sample II was obtained from $MoO_3$ and the stoichiometric amount of metallic Mo, and sample III was obtained from $MoO_3$ with 200 % excess Mo. The error bars are from the Rietveld refinement of the synchrotron data (ESRF, ID22).

| synthesis | Sample I | Sample II | Sample III |
|---|---|---|---|
| | | lattice parameters | |
| $a$ (Å) | 8.21618(3) | 8.21151(3) | 8.20886(7) |
| $b$ (Å) | 5.27262(2) | 5.27310(2) | 5.27429(4) |
| $c$ (Å) | 7.82397(2) | 7.82280(3) | 7.81971(6) |
| $\beta$ (°) | 94.6661(2) | 94.7082(3) | 94.7207(3) |
| | | atomic positions | |
| $x$ [Ba] | 0 | 0 | 0 |
| $y$ [Ba] | 0 | 0 | 0 |
| $z$ [Ba] | 0 | 0 | 0 |
| $x$ [Mo] | 0 | 0 | 0 |
| $y$ [Mo] | 0 | 0 | 0 |
| $z$ [Mo] | 0.5 | 0.5 | 0.5 |
| $x$ [P] | 0.1318(2) | 0.1306(3) | 0.1292(5) |
| $y$ [P] | 0.5 | 0.5 | 0.5 |
| $z$ [P] | 0.2898(2) | 0.2912(3) | 0.2920(5) |
| $x$ [O1] | 0.0255(3) | 0.01878(4) | 0.0221(6) |
| $y$ [O1] | 0.2612(4) | 0.2531(6) | 0.2609(8) |
| $z$ [O1] | 0.3112(2) | 0.3128(4) | 0.3104(6) |
| $x$ [O2] | 0.2632(4) | 0.2630(3) | 0.2619(9) |
| $y$ [O2] | 0.5 | 0.5 | 0.5 |
| $z$ [O2] | 0.4358(4) | 0.4344(6) | 0.4421(9) |
| $x$ [O3] | 0.1889(4) | 0.1862(6) | 0.1895(9) |
| $y$ [O3] | 0.5 | 0.5 | 0.5 |
| $z$ [O3] | 0.1105(4) | 0.1163(6) | 0.1102(9) |
| | | profile parameters | |
| $L_x$ | 0.098(4) | 0.0169(7) | 0.09(1) |
| $L_y$ | 7.64(8) | 6.66(8) | 10.3(2) |

TABLE S2. Refined lattice parameters using data sets collected with neutron and synchrotron diffraction at different temperatures.

| parameter | D2B (neutron) | ID22 (synchrotron) |
|---|---|---|
| $T_{measu.}$ (K) | 300 | 20 |
| $a$ (Å) | 8.2090(3) | 8.1755(4) |
| $b$ (Å) | 5.2713(2) | 5.2776(6) |
| $c$ (Å) | 7.8195(3) | 7.8228(6) |
| $\beta$ (°) | 94.678(3) | 94.8806(3) |
